# Supplementary material for: Efficient Edge AI: Deploying Convolutional Neural Networks on FPGA with the Gemmini Accelerator
Source: arXiv:2408.07404 source file (2024-08-14)
Supplement: Supplementary file 1 [file appendices.tex]

\section{FPGA parameters}
\label{appendix:hw_details}

Tables \ref{tab:gemmini_params} and \ref{tab:vta_params} provide the configuration parameters used for the Gemmini and VTA accelerators respectively\footnote{For Gemmini, visit \url{https://github.com/ucb-bar/gemmini/blob/master/src/main/scala/gemmini/Configs.scala} for descriptions on each parameter. For VTA, visit \url{https://github.com/apache/tvm-vta/blob/main/hardware/chisel/src/main/scala/core/Configs.scala}.}. %The resource consumption of each FPGA implementation can be found on Table \ref{tab:hw_comparison}.

\begin{table}[t]
	\caption{Gemmini configuration parameters}
	\label{tab:gemmini_params}
	\begin{center}
		\begin{tabular}{cc} \toprule
			Parameter & Value \\
			\midrule
			DIM & 32 \\
			Dataflow & Weight Stationary \\
			Scratchpad capacity [KiB] & 512 \\
			Accumulator capacity [KiB] & 128 \\
			Scratchpad banks & 4 \\
			Accumulator banks & 2 \\
			Scratchpad ports & 2 \\
			Accumulator ports & 2 \\
			Input bits & 8 \\
			Accumulator bits & 32 \\
			Spatial array output bits & 18 \\
			Max in flight mem req & 32 \\
			\bottomrule
		\end{tabular}
	\end{center}
\end{table} 

\begin{table}[t]
	\caption{VTA default configuration parameters}
	\label{tab:vta_params}
	\begin{center}
		\begin{tabular}{cc} \toprule
			Parameter & Value \\
			\midrule
			Batch size & 1 \\
			Block in size & 16 \\
			Block out size & 16 \\
			Micro-ops buffer size [KiB] & 64\\
			Input buffer size [KiB] & 16\\
			Weights buffer size [KiB] & 8\\
			Accumulator buffer size [KiB] & 64\\
			Output buffer size [KiB] & 16\\
			Input bits & 8 \\
			Weight bits & 8 \\
			Micro-ops bits & 32 \\
			Accumulator bits & 32 \\
			Output bits & 8 \\
			\bottomrule
		\end{tabular}
	\end{center}
\end{table}
